# Supplementary material for: Introducing Neural Bag of Whole-Words with ColBERTer: Contextualized Late Interactions using Enhanced Reduction
Source: arXiv:2203.13088 source file (2022-03-24)
Supplement: Supplementary file 1 [file 8.appendix-ood.tex]

%\section{Out-of-Domain Raw Results}
